# Supplementary material for: Existence of spot and lane stationary solutions for an ant active matter PDE model
Source: arXiv:2601.16820 source file (2026-01-23)
Supplement: Supplementary file 1 [file supplement.tex]

{\color{pink}
\begin{equation}
    \begin{split}
        \int_0^{2\pi} \fU^{\vK_1}_{0} \mathrm{d}\theta &= \frac{2\pi}{\lambda (\gamma + 4\pi^2k^2\sigma_c)} \left(1- \dfrac{2\pi |k| \sigma_x}{\sqrt{\lambda^2 + 4\pi^2 k^2 \sigma_x^2}}\right)\\ & \hspace{2em}+ \frac{4\pi^2 |k| \tau }{ \lambda^2(\gamma + 4\pi^2k^2\sigma_c)} \left(\frac{8\pi^2 k^2 \sigma_x^2 +  \lambda^2 }{\sqrt{\lambda^2 + 4\pi^2 k^2 \sigma_x^2}} - 4\pi|k|\sigma_x\right).
    \end{split}
\end{equation}

We have $\int_0^{2\pi}\frac{\partial_\theta \fB_{\vK_1}}{\fM_{\vK_1}}\dd\theta=\frac{2\pi k}{\mathcal{E}^c_k\lmbk}\int_0^{2\pi}\frac{-i\cos(\theta)+\tau_k\cos(2\theta)}{\sigk+i\cos(\theta)}\dd\theta$. We expand
\begin{align*}
    \int_0^{2\pi}\frac{-i\cos(\theta)+\tau_k\cos(2\theta)}{\sigk+i\cos(\theta)}\dd\theta=& \ \int_0^{2\pi}\frac{-\cos^2(\theta)+\sigk\tauk\cos(2\theta)}{\sigk^2+\cos^2(\theta)}\dd\theta\\
    =&\int_0^{2\pi}\left(\frac{\sigk^2}{\sigk^2+\cos^2(\theta)}-1+\sigk\tauk\frac{2\cos^2(\theta)-1}{\sigk^2+\cos^2(\theta)}\right)\dd\theta\\
    =&\int_0^{2\pi}\left(\frac{\sigk^2}{\sigk^2+\cos^2(\theta)}-1+2\sigk\tauk\frac{\cos^2(\theta)-\tfrac{1}{2}-\sigk^2+\sigk^2}{\sigk^2+\cos^2(\theta)}\right)\dd\theta\\
    =&\int_0^{2\pi}\left(\frac{\sigk^2-\sigk\tauk(2\sigk^2+1)}{\sigk^2+\cos^2(\theta)}+2\sigk\tauk-1\right)\dd\theta\\
    =& \ 2\pi\left(\frac{\sigk-\tauk(2\sigk^2+1)}{\sqrt{1+\sigk^2}}+2\sigk\tauk-1\right)\\
    =& \ 2\pi\left(\frac{\sigk}{\sqrt{1+\sigk^2}}-1+\tauk\left(2\sigk-\frac{2\sigk^2+1}{\sqrt{1+\sigk^2}}\right)\right)\\
    =& \ 2\pi \Aek\left(|\Azink|-1-2\tauk\sigk|\Azink|\right),
\end{align*}
using 
\begin{align*}
    \frac{1}{\Aek}\frac{1}{\sqrt{\sigk^2+1}}=& \ 2\sigk\\
    |\Azink|=& \ 2\sigk^2+1-\sqrt{(2\sigk^2+1)^2-1}.
\end{align*}
Hence, combining everything
\begin{equation*}
    \int_0^{2\pi} \fU^{\vK_1}_{0} \mathrm{d}\theta=\frac{4\pi^2 k\Aek}{\cEll\lmbk}(1-|\Azink|+2\sigk\tauk|\Azink|).
\end{equation*}
Check later.
}
